# Supplementary material for: Revisiting Local PageRank Estimation on Undirected Graphs: Simple and Optimal
Source: arXiv:2409.08978 source file (2024-09-13)
Supplement: Supplementary file 1 [file appendix.tex]

\section{Appendix} \label{sec:appendix}

\subsection{Proof of Equation}
